# Supplementary material for: Quantum versus Classical Annealing of Ising Spin Glasses
Source: arXiv:1411.5693 ancillary file (2014-11-20)
Supplement: Supplementary file 1 [file supplementary.pdf]

# Supplementary material for "Quantum Annealing versus Classical Annealing of Ising Spin Glasses"

Bettina Heim,[1] Troels F. Rønnow,[1] Sergei V. Isakov,[2] and Matthias Troyer*[1]
[1] *Theoretische Physik, ETH Zurich, 8093 Zurich, Switzerland*
[2] *Google, Brandschenkestrasse 110, 8002 Zurich, Switzerland*

## SIMULATION DETAILS

### Simulated Annealing

Simulated annealing is performed using single spin flips and the Metropolis algorithm with two different annealing schedules. We linearly decreased the temperature from $T = 3$ to zero as a function of time for Fig. 2 in the main text as in Ref. [1]. The other results were obtained for a linear increase of the inverse temperature from $\beta = 1/3$ to $\beta = 10$. We checked that both schedules produce very similar results.

### Simulated Quantum Annealing

To perform path integral QMC simulations we split the inverse temperature $\beta = 1/k_B T$ into $M$ "imaginary time" steps $\Delta_\tau = \beta/M$ and apply a Trotter-Suzuki decomposition [2, 3] to the thermal density matrix $\exp(-\beta H_q) = \exp(-\Delta_\tau H_q)^M$. This results in a mapping of the partition function of the quantum system to that of a classical system consisting of a stack of $M$ replicas of the original system. Each of these replicas corresponds to one imaginary time step in DT-SQA. Within each replica the spins are coupled by renormalized Ising couplings $J_{ij}/M$ and the transverse field gives rise to an additional "time-like" Ising coupling of strength $J_\tau = -\frac{1}{2\beta} \log \tanh \Gamma\Delta_\tau$ between spins in adjacent replicas.
In both DT-SQA and CT-SQA we perform cluster flips of segments in imaginary time for better efficiency and use periodic boundary conditions in all directions. For any finite temperature, the probability to form clusters of length $\tau$ in CT-SQA is simply given by taking the limit $M \to \infty$ of the probability to form $\tau \cdot M$ bonds along the imaginary time axis in DT-SQA. The times $t_i \in (0, 1]$, which divide adjacent clusters of the same spin orientation, can thus be generated directly according to the exponential distribution $f(\tau) = \frac{1}{\beta\Gamma} e^{-\beta\Gamma\tau}$.
Thermal equilibrium properties of the quantum system can be sampled by simulating this equivalent classical system, and SQA can be performed by varying the transverse field strength $\Gamma(t)$, which changes the coupling between time slices. In our simulations, the transverse field $\Gamma$ is decreased linearly from $\Gamma(0) = 2.5$ to zero.

## ADDITIONAL DATA

The results shown in Fig. 4B in the main text are obtained with DT-SQA, where the Trotter number $M$ has been chosen large enough for convergence to the continuous time limit. We used 1984 Trotter slices for $\beta = 128$, 768 for $\beta = 64$, 256 for $\beta = 32$, 128 for $\beta = 16$ and 64 for all lower values of $\beta$. Our estimate on the required number of Trotter slices is based on the convergence at $M = 128$ for $\beta = 20$ shown in Fig. 3A in the main text and a scaling of the Trotter error with $\beta^3/M^2$. A comparison between Fig. 1 and Fig. 2 shows that these estimates were indeed reasonable.
As mentioned in the main text, one important issue is the calculation of the final energy. Implemented on a classical computer, we can choose the configuration with the lowest energy along the imaginary time axis to improve the results. This was done for all figures in the main text with the exception of Fig. 4B. To complement this figure, Fig. 1 shows the same DT-SQA curves as Fig. 4B in the main text, but now with this optimization implemented. The same number of Trotter slices as listed above for each value of $\beta$ has been used for Fig. 1. Whereas the performance for low temperatures and short annealing times is rather weak and increases only for longer annealing times when averaging the residual

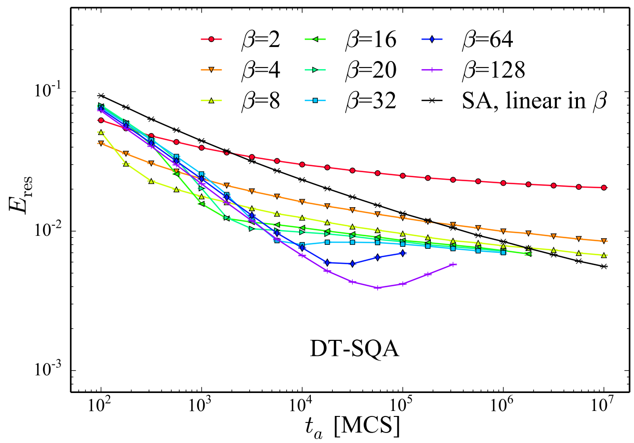


Figure 1. The minimal residual energy along imaginary time, instead of the average residual energy shown in Fig. 4B in the main text. Results are calculated for large enough $M$ to be converged to the continuous time limit and averaged over a 1000 random disorder realizations.

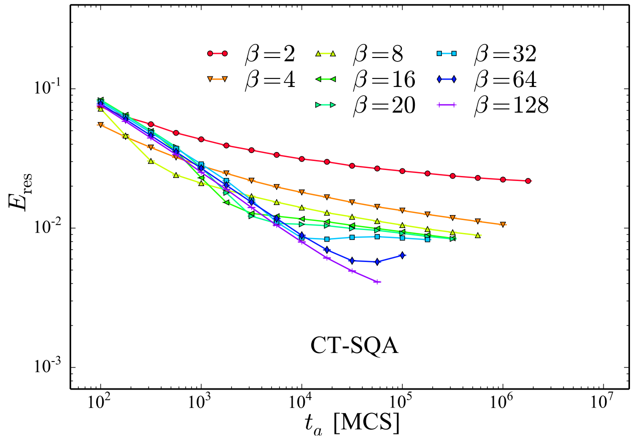


Figure 2. The dependence of the residual energy as a function of annealing time on temperature averaged over 1000 random disorder realizations using CT-SQA, complementing the DT-SQA results of Fig. 3B in the main text.

energies, no such behavior can be observed for the minimal residual energy. Compared to Fig. 4B in the main text, a slightly lower annealing temperature for a given annealing time is thus needed in order to get optimal results. In contrast to Fig. 4B in the main text, the scaling of the envelope seems fairly linear in Fig. 1, at least for the investigated temperatures.

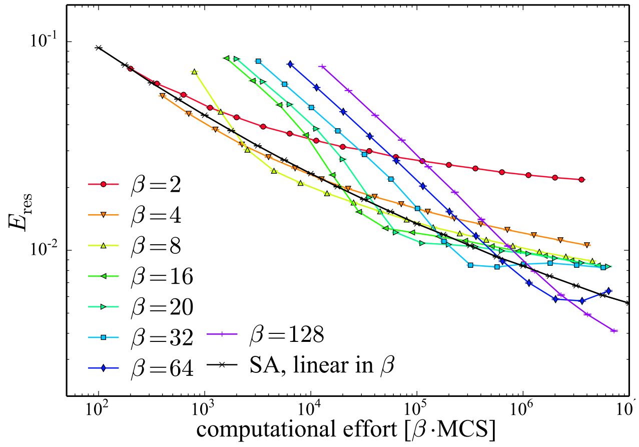


Figure 3. The residual energy as a function of computational effort averaged over 1000 random disorder realizations using CT-SQA, complementing Fig. 4A in the main text.

Complementing Fig. 3B in the main text, Fig. 2 shows the temperature dependence of the minimal residual energy with CT-SQA. Comparing the result for $\beta < 20$ shows a good correspondence between CT-SQA and DT-SQA, indicating that 64 Trotter slices are sufficient for convergence. Comparing the curves for lower temperatures, however, shows a slower decrease of the residual energy with annealing time for DT-SQA. On the other hand, the energy level at which the residual energy obtained using DT-SQA saturates is lower than that obtained with CT-SQA. This effect is more pronounced the lower the temperature.
Additionally, we provide a similar plot as in Fig. 4A in the main text using CT-SQA instead of DT-SQA. Even though the performance of CT-SQA as an optimizer is only minimally better compared to SA, Fig. 3 indicates that the discretization error is not the main reason SQA surpasses SA as a classical optimization algorithm.

## IMPLEMENTATION DETAILS

In order to make an efficient implementation of DT-SQA, we use individual bits in integer variables for storing the spins. Bit manipulations can then be used to build and update clusters along imaginary time. For each spin, we build clusters by using the algorithm in Ref. [4] to break segments of the same spin orientation into smaller pieces. At the beginning of the schedule, all Trotter slices are weakly coupled and only very small clusters are present. As the cluster size only increases significantly late during our schedule, using forward computation of the energies – saving and updating local energies – throughout the algorithm increases its performance. Finally, we approximate the exponential function as in Ref. [5]. This approximation estimates the exponential function with a relative error up to 3.5%, but if one corrects the result using a 256-element lookup table the error can be reduced to 0.01% (and 0.001% using a 4096 lookup table). We found that even a large error in the calculation of the exponential would, in general, not significantly change the behavior of the algorithm.

[1] G. E. Santoro, R. Martonak, E. Tosatti, and R. Car, Science **295**, 2427 (2002).
[2] H. F. Trotter, Proceedings of the American Mathematical Society **10**, 545 (1959).
[3] M. Suzuki, Communications in Mathematical Physics **51**, 183 (1976).
[4] L. Pierre, T. Giamarchi, and H. Schulz, Journal of Statistical Physics **48**, 135 (1987).
[5] N. N. Schraudolph, Neural Computation **11**, 853 (1999).
